# Supplementary material for: Jet Propagation and Mach-Cone Formation in (3+1)-dimensional Ideal Hydrodynamics
Source: arXiv:0910.4114 source file (2009-10-20)
Supplement: Supplementary file 1 [file appendix05.tex]

\chapter[Implementation of a Souce Term into SHASTA]
{Implementation of a Souce Term into SHASTA}
\label{SourceSHASTA}
Though the procedure the SHASTA algorithm uses shall not be reviewed in detail (for a detailed 
description see Refs.\ \cite{Rischke:1995ir,Gyulassy:1996br}), it should briefly be illustrated 
which modifications have to be taken into account to solve the energy-momentum conservation 
equations including a source term $J^\nu$
\begin{eqnarray}
\partial_\mu T^{\mu\nu}&=&J^\nu\,.
\end{eqnarray}  
Defining $T^{00}=E$ and $T^{0i}=\vec{M}$, these equations take the form, see Eqs.\ (\ref{DGL1}) 
-- (\ref{DGL2})
\begin{eqnarray}
\frac{\partial E}{\partial t} + \vec{\nabla}\cdot(E\vec{v})&=&-\vec{\nabla}\cdot(p\vec{v})+J^0\\
\frac{\partial \vec{M}}{\partial t}+\vec{\nabla}\cdot(\vec{M}\vec{v})&=&-\vec{\nabla}p+J^i\,.
\end{eqnarray}
Re-writing this into components results in
\begin{eqnarray}
\hspace*{-0.9cm}\partial_t E +\partial_x(E v_x)+\partial_y(E v_y)+\partial_z(E v_z)&=&
-\partial_x(p v_x)\nonumber\\&&-\partial_y(p v_y)-\partial_z(p v_z)+J^0\,,\nonumber\\
\hspace*{-0.9cm}\partial_t M_x +\partial_x(M_x v_x)+\partial_y(M_x v_y) + \partial_z (M_x v_z)&=&
-\partial_x p_x + J_x\,,\nonumber\\
\hspace*{-0.9cm}\partial_t M_y +\partial_x(M_y v_x)+\partial_y(M_y v_y) + \partial_z (M_y v_z)&=&
-\partial_y p_y + J_y\,,\nonumber\\
\hspace*{-0.9cm}\partial_t M_z +\partial_x(M_z v_x)+\partial_y(M_z v_y) + \partial_z (M_z v_z)&=&
-\partial_z p_z + J_z\,.
\end{eqnarray}
The SHASTA algorithm \cite{BorisBook1,BorisBook2} is based on the so-called operator splitting
method, thus it divides the evolution for each timestep into separate propagations into the $x,y$ 
and $z$-directions, implying that first the following set of equations
\begin{eqnarray}
\partial_t E +\partial_x(E v_x)&=&-\partial_x(p v_x)+J^0/3\,,\nonumber\\
\partial_t M_x +\partial_x(M_x v_x)&=&-\partial_x p_x + J_x/3\,,\nonumber\\
\partial_t M_y +\partial_x(M_y v_x)&=&J_y/3\,,\nonumber\\
\partial_t M_z +\partial_x(M_z v_x)&=&J_z/3\,,
\end{eqnarray}
corresponding to the transport of the hydrodynamic fields in the $x$-direction have to be solved 
and with the solutions to this set of equations, one solves 
\begin{eqnarray}
\partial_t E +\partial_y(E v_y)&=&-\partial_y(p v_y)+J^0/3\,,\nonumber\\
\partial_t M_x +\partial_y(M_x v_y)&=&J_x/3\,,\nonumber\\
\partial_t M_y +\partial_y(M_y v_y)&=&-\partial_y p_y + J_y/3\,,\nonumber\\
\partial_t M_z +\partial_y(M_z v_y)&=&J_z/3\,.
\end{eqnarray}
Eventually the last set of equations 
\begin{eqnarray}
\partial_t E +\partial_z(E v_z)&=&-\partial_z(p v_z)+J^0/3\,,\nonumber\\
\partial_t M_x +\partial_z(M_x v_z)&=&J_x/3\,,\nonumber\\
\partial_t M_y +\partial_z(M_y v_z)&=&J_y/3\,,\nonumber\\
\partial_t M_z +\partial_z(M_z v_z)&=&-\partial_z p_z + J_z/3\,.
\end{eqnarray}
is determined. Since these propagations are done within one timestep, there may only be added a 
third of the source term in each set of equations. \\
Generally, the SHASTA algorithms solves numerically equations of the type [see Eq.\ 
(\ref{BasicSHASTA})]
\begin{eqnarray}
\partial_t U &=& -\partial_x(Uv+f)\,.
\end{eqnarray}
The first step of the algorithm implies to computes the transported and diffused quantities 
\begin{eqnarray}
\tilde{U}_j&=&U_j-\Delta t(\partial_x U_v)+\lambda\Delta f
\end{eqnarray}
with the parameter $\lambda=\Delta t/\Delta x < 1$ given by the Courant--Friedrichs--Lewy (CFL) 
criterion \cite{CFLTheorem}, ensuring causality. Therefore, an additional source term $J$
\begin{eqnarray}
\partial_t U &=& -\partial_x(Uv+f)+J
\end{eqnarray}
leads to modified transported and diffused quantities
\begin{eqnarray}
\tilde{U}_j&=&U_j-\Delta t(\partial_x U_v)+\lambda\Delta f+\Delta t J\,.
\end{eqnarray}
Subsequently, the procedure as discussed in \cite{Rischke:1995ir} is further applied to determine 
the evolution of the hydrodynamic fields.
